# Supplementary material for: Novel View Synthesis with View-Dependent Effects from a Single Image
Source: arXiv:2312.08071 source file (2023-12-13)
Supplement: Supplementary file 1 [file X_suppl.tex]

\clearpage
\setcounter{page}{1}
\maketitlesupplementary

\section{Introduction}

We present additional details, experimental results, and visualizations that are essential to prove our NVSVDE-Net can learn to model and render novel views with view-dependent effects (VDEs). 

In Section \ref{sec:epipolar_proj}, we provide additional details on the epipolar projection equations that are used for the projection operations in our relaxed approximation of volumetric rendering. For reproducibility, in Section \ref{sec:backbone}, we provide the details of our network backbones in our NVSVDE-net. In Section \ref{sec:posenet}, we provide the details of our improved camera pose estimation network.

In Section \ref{sec:vis_vde} we provide additional visualizations of VDE modeled from \textit{single image inputs}. In Section \ref{sec:vis_nvs} we provide additional results on NVS from a single image and compare them against Single-view MPIs \cite{single_view_mpi}, PixelNeRF \cite{pixelnerf}, MINE \cite{mine}, BehindScenes \cite{behindScenes}, and SceneRF \cite{scenerf}. In Section \ref{sec:vis_inter}, we provide additional visualizations of intermediate network outputs, such as the coarse NVS output, the mean sample distance estimated by the sampler MLP head, and the changes in geometry and VDE weights induced by different camera motions.

In addition to the qualitative results presented in this supplemental, we also attach videos that better show our VDEs and Novel Views against the previous methods (these are also available in \url{https://shorturl.at/ABIJ3}). Furthermore, we complement the results in our main paper by providing videos for our qualitative results. We refer to these videos by FigX-video in the attached supplemental materials. Higher resolution/length videos can also be found at \url{https://shorturl.at/ltJT7}.

Finally, we push the boundaries of our model by rendering views with an impressive 40-frame disparity from the input view in Section \ref{sec:beyond} and discuss our method's limitations and failure cases in Section \ref{sec:failure}.

\section{Epipolar Projections}
\label{sec:epipolar_proj}

Our base relaxed volumetric rendering requires projected epipolar colors and probability logits. Such colors are obtained by projecting lines from the target ray sampling points at $t_i$ (or $t^*_i$) depths to the camera centers of the reference view. The color is then sampled from the intersections with the camera plane. Assuming a pinhole camera model, the coordinates of the epipolar color projection for a pixel in image $I$ are given by
\begin{equation} \label{eq:projection}
g(\bm{p}, t_i, R_c|\bm{t}_c, K) = \bm{p'}
\end{equation}
where $\bm{p'}$ is the image pixel coordinate to sample from reference image $I$ via bilinear sampling. $\bm{p'}$ is computed by: 

(i) Obtaining 3D points in world coordinates $\bm{p}_{w}$ by lifting $\bm{p}$ into the depth $t_i$ as described by
\begin{equation}
\bm{p}_{w} = t_iK^{-1}\bm{p};
\end{equation}

(ii) Getting reference camera coordinates $\bm{p}_{c_j}$ by rotating and translating the world coordinates by the reference camera extrinsics (rotation and translation). Given camera-to-world extrinsics, $\bm{p}_{c_j}$ is given by
\begin{equation}
\bm{p}_{c} = R'_c\bm{p}_{w_j} - R'_c\bm{t}_c,
\end{equation}
where $R'_c$ and $\bm{t}_c$ are the inverse camera rotation matrix and translation vector of the reference view, and

(iii) Projecting camera coordinates into reference view image coordinates, as given by 
\begin{equation}
\bm{p'} =  K \dfrac{\bm{p}_{c}}{z_{c}},
\end{equation}
where $K$ are the camera intrinsics and $z_{c}$ is the Z-axis component of $\bm{p}_{c}$.

\section{Additional Network Architecture Details}
\label{sec:backbone}

The network backbone $F_W$ extracts geometry and pixel-aligned features $W_D$ and $W_V$, consisting of an encoder-decoder network architecture with skip connections. An ImageNet \cite{imagenet} pre-trained ResNet-34 \cite{resnet} is chosen for $F_W$ for most of our experiments and design explorations, as it makes for a fast yet effective feature extractor encoder backbone. For the decoder side, we upscale the deep features via the nearest interpolation to the resolution of its skip connection, followed by a CONV-ELU-SKIP-CONV-ELU block, similar to the well-known Monodepth2 \cite{monodepth2}. However, at the decoder stage, we concatenate into the skip connection deep-encoded pixel positional information given by the relative pixel locations $(U, V)$. Pixel positional information is encoded by a 1$\times$1Conv-ELU-1$\times$1Conv (or MLP) head with 16 hidden units that encode the horizontal and vertical pixel positional information into an 8-element vector. We repeat this process until we reach the input resolution. All Conv layers in our decoder are $3\times3$ convolutions. To better assess the effects of our design choices (volumetric rendering approximations, rendering of VDE, etc.) we do not use any advanced block such as attention or dropout.
For a fair comparison, all methods in the Experiments and Results Section share the same network backbone $F_W$.

For our NVSVDE-Net, we set two output branches at the last decoder stage, one for $W_D$ and one for $W_V$, with $N$ and $N_v$ numbers of channels, respectively. Our NVSVDE-Net incorporates additional Linear-ELU-Linear MLP heads $F_D$ and $F_V$ with 32 hidden units. Finally, our Sampler  Linear-ELU-Linear-ELU-Linear MLP head with $4N$ input units and $2N^*$ output units utilizes 64 hidden units.

\section{Additional Details on our Improved PoseNet}
\label{sec:posenet}
We provide detailed descriptions of each layer in our improved PoseNet in Table \ref{tab:PoseNet}. In addition, it is worth noting that the camera pose network is not trained with random resized and cropped patches (as the NVS networks) but with full images at 1/2 resolution. The same resolution, 1/2, is used during testing.

A core feature of our improved PoseNet, is the processing of rotation-aligned images, which allows for extracting more relevant visual features. Fig. \ref{fig:rot_aligned} shows that it is much \enquote{easier} to understand the diagonal translation motion in the top scene and the Z-axis motion on the bottom scene when the images are rotation aligned. See attached \textit{RotAligned.gif} for an animated visualization.

\begin{table*}
    \small
    \centering
    \setlength{\tabcolsep}{2.5pt}
    \begin{tabular}{lllcc}
\hline
Outputs & Layer descriptions & Inputs & Channels & Feature sizes\\  
\hline
Image Encoder \\
$I$ & Input image & - & 3 & H$\times$W \\  
Conv1 & 3$\times$3Conv(s2), ELU, ResBlock & $I$ & 32 & H/2$\times$W/2 \\  
Conv2 & 3$\times$3Conv(s2), ELU, ResBlock & Conv1 & 64 & H/4$\times$W/4 \\  
Conv3 & 3$\times$3Conv(s2), ELU, ResBlock & Conv2 & 128 & H/8$\times$W/8 \\  
Conv4 & 3$\times$3Conv(s2), ELU, ResBlock & Conv3 & 128 & H/16$\times$W/16 \\
\hline
Joint Encoder \\
$I_1, I^R_2$ & Concatenated rotation aligned pair & - & 6 & H$\times$W \\  
Conv1 & 3$\times$3Conv(s2), ELU, ResBlock & $I$ & 32 & H/2$\times$W/2 \\  
Conv2 & 3$\times$3Conv(s2), ELU, ResBlock & Conv1 & 64 & H/4$\times$W/4 \\  
Conv3 & 3$\times$3Conv(s2), ELU, ResBlock & Conv2 & 128 & H/8$\times$W/8 \\  
Conv4$_{joint}$ & 3$\times$3Conv(s2), ELU, ResBlock & Conv3 & 128 & H/16$\times$W/16 \\
\hline
Pose Estimator \\
Conv5 & 3$\times$3Conv(s2), ELU, ResBlock & Conv4$_1$, Conv4$_2$ & 128 & H/32$\times$W/32 \\
Conv6 & 3$\times$3Conv(s2), ELU, ResBlock & Conv5 & 256 & H/64$\times$W/64 \\
Conv7 & 1$\times$1Conv, ELU & Conv6 & 256 & H/64$\times$W/64 \\
$R_0, \bm{t}_0$ & 1$\times$1Conv, ELU & GAP(Conv7) & 6 & 1 \\
\hline
$\Delta$ Pose Estimator \\
Conv5 & 3$\times$3Conv(s2), ELU, ResBlock & Conv4$_{joint}$, Conv4$_1$, Conv4$_2$ & 128 & H/32$\times$W/32 \\
Conv6 & 3$\times$3Conv(s2), ELU, ResBlock & Conv5 & 256 & H/64$\times$W/64 \\
Conv7 & 1$\times$1Conv, ELU & Conv6 & 256 & H/64$\times$W/64 \\
$\Delta R, \Delta \bm{t}$ & 1$\times$1Conv, ELU & GAP(Conv7), $R_0, \bm{t}_0$ & 6 & 1 \\
\hline

$I_1$ & Input image & - & 3 & H$\times$W \\ 
$I_2$ & Input image (target view in NVS) & - & 3 & H$\times$W \\  

Conv4$_1$ & Image Encoder & $I_1$ & 128 & H/16$\times$W/16 \\ 
Conv4$_2$ & Image Encoder & $I_2$ & 128 & H/16$\times$W/16 \\ 

$R_0, \bm{t}_0$ & Pose Estimator & Conv4$_1$, Conv4$_2$ & 6 & 1 \\

$I^R_2$ & $I^R_2 = I(g(R_0))$ & $I_2$, $R_0$, & 3 & H$\times$W \\

Conv4$_{joint}$ & Joint Encoder & $I_1$, $I^R_2$ & 128 & H/16$\times$W/16 \\ 

$\Delta R, \Delta \bm{t}$ & $\Delta$ Pose Estimator & Conv4$_{joint}$, Conv4$_1$, Conv4$_2$, $R_0, \bm{t}_0$ & 6 & 1 \\

$R, \bm{t}$ & $R = R_0 + \Delta R, \bm{t} = \bm{t}_0 + \Delta \bm{t}$ & $R_0, \Delta R, \bm{t}_0, \Delta \bm{t}$ & 6 & 1 \\

\hline
\end{tabular}
    \vspace*{2mm}
    \caption{Detailed network architecture of our improved PoseNet. s2: Stride of 2. GAP: Global Average Pooling. ResBlock(x): ELU(3$\times$3Conv(ELU(3$\times$3Conv)) + x). ELU: Exponential Linear Unit \cite{elu}.}
    \label{tab:PoseNet}
\end{table*}

\begin{figure}[t]
  \centering 
  \includegraphics[width=0.49\textwidth]{Figures/rot_aligned.jpg}
  % \vspace*{-6mm}
  \caption{Our improved PoseNet incorporates rotation-aligned views for improved camera pose estimation. Rotation-aligned views allow our PoseNet to extract more relevant visual features for finer pose estimation. See attached \textit{RotAligned.gif} for an animated visualization.}
  \label{fig:rot_aligned}
\end{figure}

% \subsection{Additional information on the adjustment blocks}

% This is because novel camera viewpoints represent different relative geometry distributions between the source (or input) view and the target view. For example, a relative camera motion of 5m (meters) in the Z-axis will mean that the first channel of $D^L$ will no longer represent the minimum disparity (or maximum depth) relative to the input view, but instead, +5m into the Z-axis, as $D^{L_0}$ will be projected by $d_0=d_{min}$ relative to the target view, \underline{not the input reference view}. These adjustments are carried out by the adjustment blocks $F_{\theta_1}$ and $F_{\theta_2}$, which learn an encoding of camera poses and the re-arrangement of the probability logits volumes for $D^L$ and $VDE^L$, respectively.

\section{Additional Visualization of VDEs}
\label{sec:vis_vde}
Due to their high sparsity, and low-frequency nature, VDEs such as glossy reflections are hard to visualize in still images. For this reason, we include several examples of our single-view-based VDE in the attached \textit{VDE-video.mp4} video. We kindly suggest viewing it.

\section{Additional Results on NVS from a Single Image}
\label{sec:vis_nvs}
For the sake of completeness, we also include the comparison with the previous methods of Single-view MPI \cite{single_view_mpi} and MINE \cite{mine} in this supplemental. Table \ref{tab:results_supp} shows the extended version of Table \ref{tab:results} with results for Single-view MPI and MINE which, for a fair comparison, were also trained with the same ResNet34 network backbone and under the same conditions as those methods in Section \ref{sec:experiments_results}. Again, our NVSVDE-Net outperforms in terms of all metrics by a considerable margin. Interestingly, Single-view MPI \cite{single_view_mpi} yields 0.4 dB better PSNR than SceneRF (but still 0.4 dB lower than ours) for the MC dataset, but with worse LPIPS, which is reflected in its qualitative results.

We also provide additional qualitative results on RE10 and MC in Figs. \ref{fig:supp_re10k} and \ref{fig:supp_mc}.
Single-view MPI \cite{single_view_mpi} and MINE \cite{mine} methods attempt to solve a very ill-posed problem of estimating densities and colors for all pixels in all image planes in the MPIs but yield very blurred results, as shown in Figs. \ref{fig:supp_re10k} and \ref{fig:supp_mc}. In contrast, our NVSVDE-Net with a \enquote{relaxed} volumetric rendering approximation yields the sharpest novel views with baked-in view-dependent effects. To complement Figs. \ref{fig:supp_re10k} and \ref{fig:supp_mc} we also attach  \textit{RE10k-results.mp4} and \textit{MC-results.mp4} videos in this supplementary materials. We kindly suggest to view them. As can be observed in the third sample of \textit{RE10k-results.mp4}, previous methods either provide blurred results for the highly reflective regions (such as Single-view MPI and MINE) or completely warps the reflective surface (such as SceneRF) instead of modeling VDEs from a single image. It is worth noting that the warping in methods such as SceneRF is due to the method modeling the reflections to be at the symmetrical \enquote{mirror} depth, which causes reflections to be considered as located farther than the reflective surface. In contrast, our NVSVDE-Net infuses VDEs into the input images (last column of \textit{RE10k-results.mp4}) and then synthesizes novel views based on our relaxed volumetric rendering approximation.

As shown in Fig. \ref{fig:supp_mc} and Video \textit{MC-results.mp4}, our NVSVDE-Net generates the highest quality of novel views, even for complex camera motions such as those in the second and third rows.

\subsection{Additional Qualitative Results on Ablation Studies}
\label{sec:supp_ablation}
Fig. \ref{fig:supp_backbones} shows results for our NVSVDE-Net with different network encoder backbones for $F_W$. Interestingly, even though our NVSVDE-Net (Swin-t) does not yield the highest PSNR in Table \ref{tab:ablations}, it presents the most discriminative VDE activation maps and the most detailed depth maps, suggesting further improvements could be achieved by fine-tuning the network architecture design. In contrast, the NVSVDE-Net (R18), which incorporates a weaker encoder backbone, struggles to predict VDE activation maps focusing on the reflective scene regions.

\begin{figure*}[t]
  \centering 
  \includegraphics[width=1.0\textwidth]{Figures/re10k_results_supp.jpg}
  % \vspace*{-7mm}
  \caption{Additional Results on the RE10k \cite{mpi} dataset. Previous methods struggle to render sharp structures for very close-by objects and reflective regions. Our NVSVDE-Net with explicitly modeled view-dependent effects (VDE) and fine-grained relaxed volumetric rendering yields more detailed synthetic views in all image regions.}
  \label{fig:supp_re10k}
\end{figure*}

\begin{figure*}[t]
  \centering 
  \includegraphics[width=1.0\textwidth]{Figures/mc_results_supp.jpg}
  % \vspace*{-7mm}
  \caption{Additional Results on the MC \cite{MCData} dataset.}
  \label{fig:supp_mc}
\end{figure*}

\begin{figure*}[t]
  \centering 
  \includegraphics[width=1.0\textwidth]{Figures/supp_backbones.jpg}
  % \vspace*{-7mm}
  \caption{Qualitative comparison among different network backbones for our NVSVDE-Net. The Swin-t \cite{swint} backbone yields more discriminative VDE activation maps $\hat{V}$ that better focus on the most reflective surfaces in the input image and relatively more detailed input view geometries $\hat{D}$.}
  \label{fig:supp_backbones}
\end{figure*}

\begin{table}
    \scriptsize
    \centering
    \setlength{\tabcolsep}{3pt}
    
\begin{tabular}{lcccccc}
\hline
Methods & VDE & MAE$\downarrow$ & PSNR$\uparrow$ & PSNR$_{lf}$$\uparrow$ & SSIM$\uparrow$ & LPIPS$\downarrow$ \\ 
\hline
\multicolumn{7}{c}{RealEstate10k (RE10k) \cite{mpi} Dataset \cite{mpi}} \\

PixelNerf \cite{pixelnerf} & No & 0.0417 & 22.8455  & 28.0945 & 0.7818 & 0.3256 \\

BehindScenes \cite{behindScenes} & No & 0.0466 & 22.9949  & 28.5941 & 0.8068 & 0.2762 \\

MINE \cite{mine} & No & 0.0415 & 23.1657  & 27.8785 & 0.8041 & 0.2976 \\

Single-view MPI \cite{single_view_mpi} & No & 0.0374 & 23.6260  & 28.9447 & 0.8112 & 0.2925 \\

SceneRF \cite{scenerf} & No & 0.0373 & 23.6087  & 28.9636 & 0.8130 & 0.2709 \\

\textbf{NVSVDE-Net (Ours)} & \textbf{Yes} & \textbf{0.0319} & \textbf{24.3131}  & \textbf{30.2529} & \textbf{0.8397} & \textbf{0.2325} \\

\hline
\multicolumn{7}{c}{MannequinChallenge (MC) Dataset \cite{MCData}} \\

PixelNerf \cite{pixelnerf} & No & 0.0511 & 21.3047  & 25.2781 & 0.7580 & 0.3455 \\

BHindScenes \cite{behindScenes} & No & 0.0463 & 21.4307  & 25.9280 & 0.7831 & 0.3101 \\

SceneRF \cite{scenerf} & No & 0.0467 & 21.5992 & 25.8119 & 0.7796 & 0.3080 \\

MINE \cite{mine} & No & 0.0487 & 21.6922  & 25.6230 & 0.7803 & 0.3306 \\

Single-view MPI \cite{single_view_mpi} & No & 0.0460 & 22.0378  & 26.2500 & 0.7873 & 0.3251 \\

\textbf{NVSVDE-Net (Ours)} & \textbf{Yes} & \textbf{0.0405} & \textbf{22.4274}  & \textbf{27.0263} & \textbf{0.8130} & \textbf{0.2733} \\

\hline
\end{tabular}
    % \vspace{-3mm}
    \caption{Single view-based NVS results. $\downarrow$/$\uparrow$ denotes the lower/higher, the better.}
    \label{tab:results_supp}
\end{table}

\section{Additional Visualizations of Intermediate Network Outputs}
\label{sec:vis_inter}
Fig. \ref{fig:intermediate} depicts the different intermediate network outputs in our NVSVDE-Net. We show the infused VDEs and VDE activation map in $I^v_{+1}$ and $\hat{V}$ respectively for a positive Z-axis camera translation in the first row. In the second row, Fig. \ref{fig:intermediate} shows a comparison between our coarse synthetic view $I''_{+1}$ and the final rendered view $I'_{+1}$. Note that the fine-grained ray sampling in $I'_{+1}$ fixes the double edge artifacts in $I''_{+1}$.

The third row of Fig. \ref{fig:intermediate} depicts the estimated geometry (inverse depth) of the input view $\hat{D}$, the mean sample distance $\overline{t}$ for the coarse synthetic view (a constant due to uniform sampling), the mean estimated sample distance $\overline{t^*}$, and the novel view geometry $\hat{D}_{+1}$. $\overline{t^*}$ resembles the scene disparity, which shows that ray samples are being taken around the highest-density regions in the scene. The novel view geometry $\hat{D}_{+1}$ can be estimated from the fine-grained ray sampling distances and weights by
\begin{equation}\label{eq:nv_geo}
\hat{D}_{c}(\bm{p}) = t^*(\bm{p}) \cdot w^*(\bm{w}).
\end{equation}

In Fig. \ref{fig:intermediate}, $+1$ sub-index represents a view 8 frames apart from the input image $I$.

We also show the effects of the so-called re-calibration blocks $F_D$ and $F_V$ in our NVSVDE-Net. While the changes in $\hat{V}$ by $F_V$ can be better visualized in the attached \textit{Extreme-NVS.mp4} video, the changes in $D^L$ are depicted in Fig. \ref{fig:supp_recal}. Fig. \ref{fig:supp_recal}. shows the corresponding channels of $D^L$ for rendering two different novel views, one with negative Z-axis motion (left column) and the other with positive Z-axis motion (right column). From top to bottom, $D^L$ channels represent the weights for close and far-away ray points. As can be noted, $F_D$ changes the values in $D_L$ to account for the novel camera view. For instance, the chair in row 3 of Fig. \ref{fig:supp_recal} is assigned less weight for the left column, as it will be further away in the novel view. Similarly, the chair is assigned more weight in row 3 for the right column, where the chair will be closer to the positive Z-axis motion novel view.

\begin{figure}
  \centering 
  \includegraphics[width=0.49\textwidth]{Figures/supp_recalib.jpg}
  \vspace*{-6mm}
  \caption{Visualization of the effects of the adjustment MLP block $F_D$. Differences in channel activations of $D^L$ show the re-calibration carried by $F_D$ for rendering novel view geometry at the target camera views.}
  \label{fig:supp_recal}
\end{figure}

\begin{figure*}[t]
  \centering 
  \includegraphics[width=1.0\textwidth]{Figures/intermediate.jpg}
  % \vspace*{-7mm}
  \caption{Intermediate outputs of our NVSVDE-Net}
  \label{fig:intermediate}
\end{figure*}

\section{Rendering Views Beyond the Training Set}
\label{sec:beyond}
We trained our NVSVDE-Net to render views that are at most 16 frames apart from the single-image input. In this experiment, we render views equivalent to 40 frames apart from the input view and show our results in the attached \textit{Extreme-NVS.mp4} video. We cordially invite the reader to observe the video, also available at the following anonymous repository link: \url{https://shorturl.at/ABIJ3}. Despite the inherent challenges associated with extreme Novel View Synthesis (NVS), our method consistently produces realistic views, albeit with certain observable artifacts, as anticipated in any single-view NVS framework.

The \textit{Extreme-NVS.mp4} video illustrates two primary failure scenarios. Firstly, when the camera motion exceeds a certain threshold, our relaxed volumetric rendering encounters challenges in modeling large dis-occluded regions, a known issue prevalent in prior methods relying on projections for rendering \cite{single_view_mpi, pixelnerf, mine, behindScenes, scenerf}. Generative models have effectively addressed this concern but very often show stochastic artifacts. Secondly, under substantial camera motions, our negative disparity-based view-dependent effects (VDEs) struggle to model reflections accurately, leaking incorrect colors into the scene. Addressing this challenge may involve incorporating extreme NVS samples during training and refining the regularization applied to the intermediate output $I^v_c$ of the VDE-infused input image.

\section{Limitations and Failure Cases}
\label{sec:failure}
The architecture of our NVSVDE-Net, as defined in Eq. \ref{eq:vde_syn}, imposes limitations on rendering high-frequency view-dependent appearances. This, however, proves to be adequate for rendering most glossy reflections in the context of realistic NVS. Future avenues of research will explore the modeling of both low- and high-frequency View-Dependent Embeddings from a single image to mitigate this inherent limitation.

Another limitation of our approach is apparent when dealing with extreme NVS scenarios, where novel views with baselines significantly surpassing those encountered during training are required. As demonstrated in Section \ref{sec:beyond}, our network encounters challenges in generating artifact-free novel views when tasked with rendering views 40 frames apart from the input view, a significant departure from the training set's 16-frame disparity. The impediments arise from the sheer size of occlusions, rendering them impractical to inpaint through projected colors, and the limited context available to the sampler MLP head for predicting sampling distances from the few valid projected $D^L$ and $I^v_c$ values. Future research directions include incorporating generative model properties into our NVSVDE-Net for realistic wide-baseline occlusion inpainting.
