# Supplementary material for: Novel View Synthesis with View-Dependent Effects from a Single Image
Source: arXiv:2312.08071 source file (2023-12-13)
Supplement: Supplementary file 2 [file table_supp.tex]

\begin{tabular}{lcccccc}
\hline
Methods & VDE & MAE$\downarrow$ & PSNR$\uparrow$ & PSNR$_{lf}$$\uparrow$ & SSIM$\uparrow$ & LPIPS$\downarrow$ \\ 
\hline
\multicolumn{7}{c}{RealEstate10k (RE10k) \cite{mpi} Dataset \cite{mpi}} \\

PixelNerf \cite{pixelnerf} & No & 0.0417 & 22.8455  & 28.0945 & 0.7818 & 0.3256 \\

BehindScenes \cite{behindScenes} & No & 0.0466 & 22.9949  & 28.5941 & 0.8068 & 0.2762 \\

MINE \cite{mine} & No & 0.0415 & 23.1657  & 27.8785 & 0.8041 & 0.2976 \\

Single-view MPI \cite{single_view_mpi} & No & 0.0374 & 23.6260  & 28.9447 & 0.8112 & 0.2925 \\

SceneRF \cite{scenerf} & No & 0.0373 & 23.6087  & 28.9636 & 0.8130 & 0.2709 \\

\textbf{NVSVDE-Net (Ours)} & \textbf{Yes} & \textbf{0.0319} & \textbf{24.3131}  & \textbf{30.2529} & \textbf{0.8397} & \textbf{0.2325} \\

\hline
\multicolumn{7}{c}{MannequinChallenge (MC) Dataset \cite{MCData}} \\

PixelNerf \cite{pixelnerf} & No & 0.0511 & 21.3047  & 25.2781 & 0.7580 & 0.3455 \\

BHindScenes \cite{behindScenes} & No & 0.0463 & 21.4307  & 25.9280 & 0.7831 & 0.3101 \\

SceneRF \cite{scenerf} & No & 0.0467 & 21.5992 & 25.8119 & 0.7796 & 0.3080 \\

MINE \cite{mine} & No & 0.0487 & 21.6922  & 25.6230 & 0.7803 & 0.3306 \\

Single-view MPI \cite{single_view_mpi} & No & 0.0460 & 22.0378  & 26.2500 & 0.7873 & 0.3251 \\

\textbf{NVSVDE-Net (Ours)} & \textbf{Yes} & \textbf{0.0405} & \textbf{22.4274}  & \textbf{27.0263} & \textbf{0.8130} & \textbf{0.2733} \\

\hline
\end{tabular}
